# Supplementary material for: Ground-state cooling of a mechanical oscillator by heating
Source: arXiv:2306.15746 ancillary file (2023-06-27)
Supplement: Supplementary file 1 [file SI.pdf]

# Supplemental Material for “Ground-state cooling of a mechanical oscillator by heating”

Cheng Wang<sup>1</sup>, Louise Banniard<sup>1</sup>, Kjetil Børkje<sup>2</sup>, Francesco

Massel<sup>2</sup>, Laure Mercier de Lépinay<sup>1</sup> and Mika A. Sillanpää<sup>1</sup>

<sup>1</sup> *Department of Applied Physics, Aalto University, FI-00076 Aalto, Finland*

<sup>2</sup> *Department of Science and Industry Systems, University of South-Eastern Norway, PO Box 235, Kongsberg, Norway*

## I. THEORY

### A. Model

We start from the quantum Langevin equations

$$\dot{a} = -\left(\frac{\kappa}{2} + i\omega_c\right)a - ig_0(b + b^\dagger)a + \sqrt{\kappa}\xi \quad (\text{S1})$$

$$\dot{b} = -\left(\frac{\gamma}{2} + i\omega_m\right)b - ig_0(a^\dagger a - \langle a^\dagger a \rangle) + \sqrt{\gamma}\eta \quad (\text{S2})$$

where the Gaussian thermal noise from the mechanical bath is assumed to obey [1]

$$\langle \eta^\dagger[\omega]\eta[\omega'] \rangle = n_m^T 2\pi\delta(\omega + \omega') \quad (\text{S3})$$

$$\langle \eta[\omega]\eta^\dagger[\omega'] \rangle = (n_m^T + 1) 2\pi\delta(\omega + \omega') \quad (\text{S4})$$

and  $n_m^T$  is the bath's thermal occupation number.

We also assume Gaussian input noise

$$\xi(t) = e^{-i(\omega_c - \omega_m)t} (\xi_c(t) + \xi_q(t)) \quad (\text{S5})$$

to the cavity mode, which we separate into a classical contribution  $\xi_c$  and a quantum operator  $\xi_q$ . The latter represents vacuum noise, such that  $\langle \xi_q^\dagger(t)\xi_q(t') \rangle = 0$ . To satisfy standard commutation relations, the operator  $\xi_q$  must satisfy

$$[\xi_q[\omega], \xi_q^\dagger[\omega']] = 2\pi\delta(\omega + \omega'), \quad (\text{S6})$$

where we define the Fourier transformation according to

$$f^{(\dagger)}[\omega] = \int_{-\infty}^{\infty} dt e^{i\omega t} f^{(\dagger)}(t). \quad (\text{S7})$$

Furthermore, we define

$$\langle \xi_c^*[\omega]\xi_c[\omega'] \rangle = N_{\text{in}}(-\omega) 2\pi\delta(\omega + \omega'), \quad (\text{S8})$$

such that the spectral content of the incoming noise is characterized by the function  $N_{\text{in}}$ . We will assume that the noise  $\xi_c$  has a spectrum centered around zero frequency, meaning that the incoming noise  $\xi$  is centered at the red sideband frequency

$$\omega_r = \omega_c - \omega_m, \quad (\text{S9})$$

and we will denote the classical noise bandwidth by the symbol  $\sigma$ . The simplest function satisfying these properties is the rectangular function

$$N_{\text{in}}(\omega) = 2\pi N_0 \{ \Theta[\omega + \sigma/2] - \Theta[\omega - \sigma/2] \}, \quad (\text{S10})$$

which is constant in a frequency interval of width  $\sigma$  around zero frequency and vanishes otherwise. This is a good approximation to the noise spectrum produced in the experiments, and is sufficient to explain the observed results both qualitatively and, to a large degree, quantitatively. We will assume that both the noise bandwidth and the cavity linewidth is much smaller than the mechanical resonance frequency, i.e.,

$$\kappa, \sigma \ll \omega_m, \quad (\text{S11})$$

but we make no assumptions on the ratio  $\sigma/\kappa$ .

We will additionally assume that  $\langle \xi[\omega]\xi[\omega'] \rangle = 0$ , meaning that there are no correlations between the noise at different frequencies. Whether this is true depends on how the noise is actually generated. In any case, we do not expect that deviations from this will result in significant changes to the results from the quantum-noise approach below as long as the noise bandwidth is much smaller than the mechanical resonance frequency.

### B. Quantum noise approach

In the weak coupling regime  $\gamma, \gamma_{\text{opt}} \ll \kappa$ , where the optomechanical damping rate  $\gamma_{\text{opt}}$  is to be defined, and for noise bandwidth  $\sigma \gg \gamma, \gamma_{\text{opt}}$ , we can determine the mechanical oscillator's average phonon number  $n_m$  from the quantum noise approach [1]. We define the photon number fluctuation spectrum

$$S_{\delta n \delta n}(\omega) = \int_{-\infty}^{\infty} d\tau e^{i\omega\tau} \langle \delta n(\tau) \delta n(0) \rangle, \quad (\text{S12})$$

with

$$\delta n = a^\dagger a - \langle a^\dagger a \rangle. \quad (\text{S13})$$

In the quantum noise approach, the average phonon number is given by [1, 2]

$$n_m = \frac{\gamma n_m^T + \gamma_{\text{opt}} n_{ba}}{\gamma + \gamma_{\text{opt}}} \quad (\text{S14})$$

with

$$\gamma_{\text{opt}} = g_0^2 \left( S_{\delta n \delta n}^{(0)}(\omega_m) - S_{\delta n \delta n}^{(0)}(-\omega_m) \right), \quad (\text{S15})$$

$$n_{ba} = \frac{S_{\delta n \delta n}^{(0)}(-\omega_m)}{S_{\delta n \delta n}^{(0)}(\omega_m) - S_{\delta n \delta n}^{(0)}(-\omega_m)}, \quad (\text{S16})$$

and where  $S_{\delta n \delta n}^{(0)}(\omega)$  refers to the photon number fluctuation spectrum in absence of optomechanical coupling, i.e., for  $g_0 = 0$ .

In the absence of optomechanical coupling, the cavity annihilation operator is

$$a_0[\omega] = \sqrt{\kappa} \chi_c(\omega - \omega_r) \xi[\omega], \quad (\text{S17})$$

with the cavity susceptibility defined as

$$\chi_c(\omega) = \frac{1}{\kappa/2 - i(\omega - \omega_m)}. \quad (\text{S18})$$

Exploiting that the incoming noise is Gaussian, we can write

$$S_{\delta n \delta n}^{(0)}(\omega) = \int_{-\infty}^{\infty} \frac{d\omega_1}{2\pi} \left[ S_{a^\dagger a}^{(0)}(\omega_1) S_{aa^\dagger}^{(0)}(\omega - \omega_1) + S_{a^\dagger a^\dagger}^{(0)}(\omega_1) S_{aa}^{(0)}(\omega - \omega_1) \right] \quad (\text{S19})$$

where

$$S_{AB}^{(0)}(\omega) = \int_{-\infty}^{\infty} \frac{d\omega'}{2\pi} \langle A_0[\omega] B_0[\omega'] \rangle \quad (\text{S20})$$

and  $A$  and  $B$  are either  $a$  or  $a^\dagger$ .

Given the assumptions on the incoming noise  $\xi$ , we now find

$$S_{\delta n \delta n}^{(0)}(\omega) = \kappa^2 \int_{-\infty}^{\infty} \frac{d\omega_1}{2\pi} |\chi_c(-\omega_1)|^2 |\chi_c(\omega - \omega_1)|^2 \times N_{\text{in}}(-\omega_1) [N_{\text{in}}(\omega - \omega_1) + 1]. \quad (\text{S21})$$

This can be straightforwardly determined from the input noise spectrum  $N_{\text{in}}(\omega)$  and the cavity susceptibility  $\chi_c(\omega)$ .

We now use the noise spectrum given by Equation (S10). We first note that, in the absence of optomechanical coupling, the average cavity photon number then becomes

$$\begin{aligned} \bar{n}_0 &= \int_{-\infty}^{\infty} \frac{d\omega}{2\pi} S_{a^\dagger a}^{(0)}(\omega) = \kappa N_0 \int_{-\sigma/2}^{\sigma/2} d\omega |\chi_c(\omega)|^2 \\ &\approx \frac{\kappa \sigma N_0}{\omega_m^2} = \frac{\kappa F_0}{\omega_m^2}, \end{aligned} \quad (\text{S22})$$

where

$$F_0 = \sigma N_0 \quad (\text{S23})$$

is the total incoming photon flux.

We note that the product  $N_{\text{in}}(-\omega_1) N_{\text{in}}(\omega - \omega_1)$  in Equation (S21), which describes *stimulated* emission of sideband photons, gives no contribution when  $|\omega| > \sigma$ . Thus, for  $\omega = \pm \omega_m > \sigma$ , we get

$$\begin{aligned} S_{\delta n \delta n}^{(0)}(\omega) &= \kappa^2 N_0 \int_{-\sigma/2}^{\sigma/2} d\omega_1 |\chi_c(-\omega_1)|^2 |\chi_c(\omega - \omega_1)|^2 \\ &\approx \frac{\kappa^2 N_0}{\omega_m^2} \int_{-\sigma/2}^{\sigma/2} d\omega_1 |\chi_c(\omega - \omega_1)|^2 \end{aligned} \quad (\text{S24})$$

in the limit (S11). For  $\omega = -\omega_m$ , this gives

$$S_{\delta n \delta n}^{(0)}(-\omega_m) \approx \frac{\kappa^2 F_0}{4\omega_m^4}, \quad (\text{S25})$$

whereas for  $\omega = +\omega_m$ , we get

$$S_{\delta n \delta n}^{(0)}(\omega_m) \approx \frac{2\pi\kappa F_0}{\omega_m^2 \sigma} f\left(\frac{\sigma}{\kappa}\right), \quad (\text{S26})$$

when defining

$$f\left(\frac{\sigma}{\kappa}\right) = \frac{2}{\pi} \arctan\left(\frac{\sigma}{\kappa}\right). \quad (\text{S27})$$

We note that  $f(\sigma/\kappa) \approx 1$  for large bandwidths  $\sigma/\kappa \gg 1$ , and that  $f(\sigma/\kappa) \approx 2\sigma/(\pi\kappa)$  for small bandwidths  $\sigma/\kappa \ll 1$ .

From Equation (S15), the optomechanical damping rate now becomes

$$\gamma_{\text{opt}} = \frac{g_0^2 \kappa F_0}{\omega_m^2 \sigma} \left[ 2\pi f\left(\frac{\sigma}{\kappa}\right) - \frac{\kappa \sigma}{(2\omega_m)^2} \right] \quad (\text{S28})$$

For small bandwidths  $\sigma/\kappa \ll 1$  compared to the cavity linewidth, this becomes

$$\gamma_{\text{opt}} \approx \frac{4g_0^2 F_0}{\omega_m^2} \approx \frac{4G^2}{\kappa} \quad (\text{S29})$$

with  $G = g_0 \sqrt{\bar{n}_0}$ . This is just like the optomechanical damping rate familiar from coherent driving at the red sideband in the resolved sideband regime  $\kappa/\omega_m \ll 1$ , where  $G$  is the enhanced optomechanical coupling proportional to the square root of the average cavity photon number. Conversely, for large bandwidths  $\sigma/\kappa \gg 1$ , we find

$$\gamma_{\text{opt}} \approx \frac{2\pi g_0^2 \kappa F_0}{\omega_m^2 \sigma} \approx \frac{2\pi G^2}{\sigma}. \quad (\text{S30})$$

The above approximate expressions tells us that, *for a constant input flux  $F_0$* , the damping rate is constant in the small bandwidth regime  $\sigma/\kappa \ll 1$ , but is reduced by a factor  $\pi\kappa/(2\sigma)$  in the large bandwidth regime  $\sigma/\kappa \gg 1$ . In Figure S1, we plot the approximate damping rate

$$\gamma_{\text{opt}} \approx \frac{4g_0^2 F_0}{\omega_m^2} \cdot \frac{\pi\kappa}{2\sigma} f\left(\frac{\sigma}{\kappa}\right) \quad (\text{S31})$$

as a function of  $\sigma/\kappa$  for fixed input flux  $F_0$ .

The quantum limit to the phonon number given by Equation (S16) becomes

$$\begin{aligned} n_{ba} &\approx \frac{S_{\delta n \delta n}^{(0)}(-\omega_m)}{S_{\delta n \delta n}^{(0)}(\omega_m)} \\ &\approx \frac{\kappa \sigma}{8\pi \omega_m^2 f(\sigma/\kappa)}. \end{aligned} \quad (\text{S32})$$

For small bandwidth  $\sigma/\kappa \ll 1$ , this reduces to the limit  $n_{ba} = (\kappa/4\omega_m)^2$  familiar from coherent driving [2, 3], whereas for large bandwidths  $\sigma/\kappa \gg 1$ , it increases to  $n_{ba} = \kappa\sigma/(8\pi\omega_m^2)$ , which is still much smaller than 1 with our assumptions.

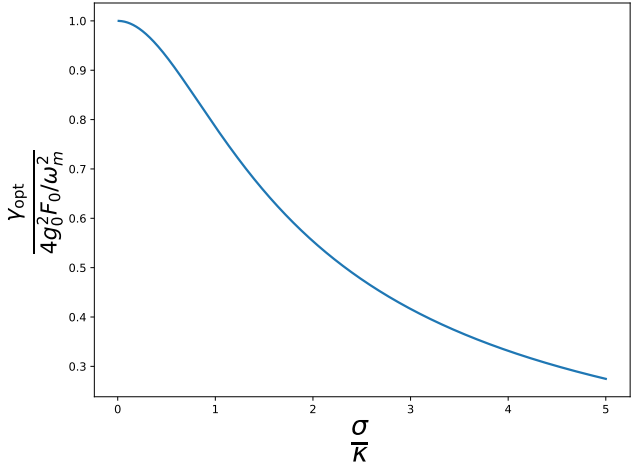

FIG. S1. Approximate optomechanical damping rate as a function of  $\sigma/\kappa$  for the rectangular noise model and for fixed input flux  $F_0$ .

### C. Beyond the quantum noise approach

The quantum noise approach is no longer applicable when the noise bandwidth  $\sigma$  becomes so small as to be comparable to the effective mechanical linewidth  $\gamma_{\text{eff}} = \gamma + \gamma_{\text{opt}}$ . To address the low bandwidth regime, let us now go back to the equations of motion (S1) and (S2). Assuming that  $\xi_{\text{cl}}(t)$  varies slowly on the timescale  $1/\kappa$ , i.e., that the noise bandwidth  $\sigma$  is small compared to the cavity linewidth  $\kappa$ , we can write a linearized solution for the cavity field as

$$a(t) \approx e^{-i\omega_r t} \left[ a_0(t) - ig_0 \int_{-\infty}^t d\tau e^{-(\kappa/2 + i\omega_m)(t-\tau)} (b(\tau) + b^\dagger(\tau)) a_0(\tau) \right], \quad (\text{S33})$$

where

$$a_0(t) \approx \frac{\sqrt{\kappa}\xi_c(t)}{\kappa/2 + i\omega_m} + \zeta_q(t) \quad (\text{S34})$$

is the approximate solution, in a frame rotating at  $\omega_r$ , in absence of optomechanical coupling and where

$$\zeta_q(t) = \int_{-\infty}^t d\tau e^{-(\kappa/2 + i\omega_m)(t-\tau)} \sqrt{\kappa}\xi_q(\tau). \quad (\text{S35})$$

The equation of motion for the phonon annihilation operator is then approximately given by

$$\begin{aligned} \dot{b} \approx & -\left(\frac{\gamma}{2} + i\omega_m\right)b - \frac{2g_0^2}{\omega_m^2}\xi_c^*(t)\xi_c(t)b \\ & + \sqrt{\gamma}\eta - ig_0 \left( \frac{\sqrt{\kappa}\xi_c^*(t)}{\kappa/2 - i\omega_m}\zeta_q(t) + \frac{\sqrt{\kappa}\xi_c(t)}{\kappa/2 + i\omega_m}\zeta_q^\dagger(t) \right) \\ & - ig_0 \frac{\kappa}{\omega_m^2} [\xi_c^*(t)\xi_c(t) - \langle \xi_c^*(t)\xi_c(t) \rangle]. \end{aligned} \quad (\text{S36})$$

when we assume the resolved sideband regime  $\kappa \ll \omega_m$ . It is worth noting that only the classical amplitude noise  $|\xi_c|$  enters here, not the classical phase noise, which is a consequence of assuming a noise bandwidth  $\sigma \ll \kappa$ .

The last term in the first line of Equation (S36) describes optical damping of the mechanical mode. In the limit where the autocorrelation time of the noise  $\xi_c(t)$  is much shorter than the effective mechanical linewidth, we can approximate  $\xi_c^*(t)\xi_c(t) = |\xi_c(t)|^2$  by its average value here. However, this is not appropriate when the noise bandwidth is small enough to be comparable with the mechanical damping rate.

The second line of Equation (S36) describes both thermal noise and radiation pressure shot noise that can drive the mechanical resonator at its resonance frequency. The last line, however, describes low frequency noise, i.e., slow variations in the radiation pressure force experienced by the mechanical oscillator, which leads to slow variations in its equilibrium position and thereby variations in the cavity resonance frequency. However, as long as these frequency variations are sufficiently small compared to the cavity linewidth, we can ignore the last line.

Since  $\xi_c(t)$  is classical noise, i.e., commutes with itself at different times, the solution of Equation (S36) becomes

$$b(t) = \int_{-\infty}^t d\tau e^{-(\gamma/2 + i\omega_m)(t-\tau) - \Gamma(t,\tau)/2} \Lambda(\tau) \quad (\text{S37})$$

when defining

$$\Gamma(t,\tau) = \frac{4g_0^2}{\omega_m^2} \int_{\tau}^t ds \xi_c^*(s)\xi_c(s) \quad (\text{S38})$$

and

$$\begin{aligned} \Lambda(t) = & \sqrt{\gamma}\eta(t) \\ & - ig_0 \left( \frac{\sqrt{\kappa}\xi_c^*(t)}{\kappa/2 - i\omega_m}\zeta_q(t) + \frac{\sqrt{\kappa}\xi_c(t)}{\kappa/2 + i\omega_m}\zeta_q^\dagger(t) \right). \end{aligned} \quad (\text{S39})$$

In the following, we will ignore the last line in  $\Lambda(t)$  for simplicity, meaning that we ignore radiation pressure shot noise. This is a good approximation in the resolved sideband regime  $\kappa \ll \omega_m$ .

The *ensemble averaged* phonon number now becomes

$$\begin{aligned} n_m = & \langle b^\dagger(t)b(t) \rangle \\ \approx & \gamma n_m^T \int_{-\infty}^t d\tau e^{-\gamma(t-\tau)} \langle e^{-\Gamma(t,\tau)} \rangle. \end{aligned} \quad (\text{S40})$$

We also define the mechanical spectral density as

$$\begin{aligned} S_{b^\dagger b}(\omega) = & \int_{-\infty}^{\infty} d\tau e^{i\omega\tau} \langle b^\dagger(t+\tau)b(t) \rangle \\ \approx & \gamma n_m^T \int_{-\infty}^{\infty} d\tau e^{i(\omega+\omega_m)\tau} \\ & \times \int_{-\infty}^{\min(t,t+\tau)} d\tau_1 e^{-\gamma(t+\tau/2-\tau_1)} \langle e^{-[\Gamma(t+\tau,\tau_1) + \Gamma(t,\tau_1)]/2} \rangle. \end{aligned} \quad (\text{S41})$$

To evaluate the integrals in these expressions, we will need the relations

$$\langle \xi_c^*(t) \xi_c(t') \rangle = \int_{-\infty}^{\infty} \frac{d\omega}{2\pi} e^{-i\omega(t-t')} N_{\text{in}}(-\omega) \quad (\text{S42})$$

and

$$\langle \xi_c^*(t) \xi_c(t) \rangle = \int_{-\infty}^{\infty} \frac{d\omega}{2\pi} N_{\text{in}}(-\omega) = \sigma N_0 = F_0 \quad (\text{S43})$$

where  $F_0$  is the average incoming photon flux as defined in Equation (S23).

### 1. Large bandwidth limit $\sigma \gg \gamma, \gamma_{\text{opt}}$

We will start by considering the large bandwidth limit where the noise bandwidth  $\sigma$  is large compared to the optical damping rate  $\gamma_{\text{opt}}$  of the mechanical oscillator. This will allow us to derive approximate expressions for the average phonon number  $n_m$  and the effective mechanical linewidth  $\gamma_{\text{eff}}$  to first order in  $\gamma_{\text{opt}}/\sigma$ .

#### a. Average phonon number

To find an expression for the average phonon number, we start by defining

$$\gamma_{\text{opt}} = \frac{4g_0^2 F_0}{\omega_m^2}, \quad (\text{S44})$$

which is the approximate optomechanical damping rate in the large bandwidth limit  $\sigma \gg \gamma_{\text{opt}}$  (see Equation (S29)). We may then write

$$\Gamma(t, \tau) = \gamma_{\text{opt}}(t - \tau) + \frac{\gamma_{\text{opt}}}{F_0} \int_{\tau}^t ds (\xi_c^*(s) \xi_c(s) - F_0). \quad (\text{S45})$$

We now expand the exponent in (S40) to second order in the second term of (S45), which, as we will see, is equivalent to expanding in  $\gamma_{\text{opt}}/\sigma$ . This gives

$$\begin{aligned} \langle e^{-\Gamma(t, \tau)} \rangle &= e^{-\gamma_{\text{opt}}(t-\tau)} \left[ 1 + \frac{1}{2} \left( \frac{\gamma_{\text{opt}}}{F_0} \right)^2 \int_{\tau}^t ds_1 \int_{\tau}^t ds_2 \right. \\ &\quad \times \langle (\xi_c^*(s_1) \xi_c(s_1) - F_0) (\xi_c^*(s_2) \xi_c(s_2) - F_0) \rangle \Big] \\ &= e^{-\gamma_{\text{opt}}(t-\tau)} \left[ 1 + \frac{1}{2} \left( \frac{\gamma_{\text{opt}}}{F_0} \right)^2 \right. \\ &\quad \times \int_{\tau}^t ds_1 \int_{\tau}^t ds_2 \langle \xi_c^*(s_1) \xi_c(s_2) \rangle \langle \xi_c(s_1) \xi_c^*(s_2) \rangle \Big] \quad (\text{S46}) \\ &= e^{-\gamma_{\text{opt}}(t-\tau)} \left[ 1 + \frac{1}{2} \left( \frac{\gamma_{\text{opt}}}{F_0} \right)^2 \int_{-\infty}^{\infty} \frac{d\omega}{2\pi} \int_{-\infty}^{\infty} \frac{d\omega'}{2\pi} \right. \\ &\quad \times \left. \frac{\sin^2[(\omega + \omega')(t - \tau)/2]}{[(\omega + \omega')/2]^2} N_{\text{in}}(-\omega) N_{\text{in}}(\omega') \right] \end{aligned}$$

when using Wick's theorem. For small  $\gamma_{\text{opt}}/\sigma$ , we can simplify the frequency integrals by the approximation

$$\frac{\sin^2[(\omega + \omega')(t - \tau)/2]}{[(\omega + \omega')/2]^2} \rightarrow 2\pi(t - \tau)\delta(\omega + \omega'), \quad (\text{S47})$$

such that

$$\begin{aligned} \int \frac{d\omega}{2\pi} \int \frac{d\omega'}{2\pi} \frac{\sin^2[(\omega + \omega')(t - \tau)/2]}{[(\omega + \omega')/2]^2} N_{\text{in}}(-\omega) N_{\text{in}}(\omega') \\ \approx (t - \tau) \int \frac{d\omega}{2\pi} N_{\text{in}}^2(-\omega) = 2\pi N_0^2 \sigma (t - \tau). \end{aligned} \quad (\text{S48})$$

Inserting this in Equation (S46) gives

$$\langle e^{-\Gamma(t, \tau)} \rangle = e^{-\gamma_{\text{opt}}(t-\tau)} \left[ 1 + \pi \frac{\gamma_{\text{opt}}^2 (t - \tau)}{\sigma} \right] \quad (\text{S49})$$

Using

$$\int_{-\infty}^t d\tau e^{-(\gamma + \gamma_{\text{opt}})(t-\tau)} = \frac{1}{\gamma + \gamma_{\text{opt}}} \quad (\text{S50})$$

$$\int_{-\infty}^t d\tau (t - \tau) e^{-(\gamma + \gamma_{\text{opt}})(t-\tau)} = \frac{1}{(\gamma + \gamma_{\text{opt}})^2}, \quad (\text{S51})$$

the phonon number (S40) then becomes

$$\begin{aligned} n_m &\approx \frac{\gamma n_m^T}{\gamma + \gamma_{\text{opt}}} \left( 1 + \frac{\pi \gamma_{\text{opt}}^2}{(\gamma + \gamma_{\text{opt}}) \sigma} \right) \\ &= n_m^{(\text{QNA})} \left( 1 + \frac{\pi \gamma_{\text{opt}}^2}{(\gamma + \gamma_{\text{opt}}) \sigma} \right). \end{aligned} \quad (\text{S52})$$

Here,  $n_m^{(\text{QNA})}$  is the result one finds from the quantum noise approach when  $\sigma \ll \kappa \ll \omega_m$ . The second term in the paranthesis is the correction as  $\sigma$  starts to approach  $\gamma_{\text{opt}}$  from above.

#### b. Average spectrum and effective mechanical linewidth

Expanding in the fluctuations, i.e., the second term of (S45) as before, and using the same approximation (S47), gives the spectral density

$$\begin{aligned} S(\omega) &= \gamma n_m^T \int_{-\infty}^{\infty} d\tau e^{i(\omega + \omega_m)\tau} \\ &\quad \times \int_{-\infty}^{\min(t, t+\tau)} ds e^{-(\gamma + \gamma_{\text{opt}})(t+\tau/2-s)} \\ &\quad \left[ 1 + \frac{\pi \gamma_{\text{opt}}^2}{\sigma} \left( t + \frac{\tau}{2} - s \right) \right]. \end{aligned} \quad (\text{S53})$$

To lowest order in  $\gamma_{\text{opt}}/\sigma$ , the  $s$ -integral gives

$$S(\omega) = n_m \int_{-\infty}^{\infty} d\tau e^{i(\omega + \omega_m)\tau} e^{-\gamma_{\text{eff}}|\tau|/2} \quad (\text{S54})$$

with  $n_m$  as in Equation (S52) and when defining the effective mechanical damping rate

$$\gamma_{\text{eff}} = \gamma + \gamma_{\text{opt}} \left(1 - \frac{\pi\gamma_{\text{opt}}}{\sigma}\right). \quad (\text{S55})$$

Finally, evaluating the  $\tau$ -integral gives the Lorentzian spectrum

$$S(\omega) = \frac{\gamma_{\text{eff}} n_m}{(\gamma_{\text{eff}}/2)^2 + (\omega + \omega_m)^2}. \quad (\text{S56})$$

## 2. Small bandwidth limit $\sigma \ll \gamma, \gamma_{\text{opt}}$

In the regime where the noise bandwidth  $\sigma$  is the smallest rate in the problem, we can approximate (S38) by

$$\Gamma(t, \tau) \approx \frac{4g_0^2 \xi_c^*(t) \xi_c(t)}{\omega_m^2} (t - \tau), \quad (\text{S57})$$

which means that the mechanical damping follows the amplitude noise adiabatically in this regime.

We are now considering the case where the mechanical mode reaches a quasi-steady state on a time scale much faster than the scale at which the noise amplitude

$$r(t) = |\xi_c(t)| \quad (\text{S58})$$

varies. It is then useful to think about a time-dependent average phonon number, which we write

$$\langle b^\dagger(t)b(t) \rangle_{r(t)} = \frac{\gamma n_m^T}{\gamma + 4g_0^2 r^2(t)/\omega_m^2}. \quad (\text{S59})$$

This expression comes about by performing the  $\tau$ -integral in Equation (S40) while treating  $r^2(t)$  as a constant, which is appropriate if the noise bandwidth  $\sigma$  is much smaller than the thermal equilibration rate of the oscillator. As before, in order to simplify, we ignore the second term in the numerator, i.e., the heating term due to radiation pressure shot noise. We can interpret (S59) as a time-dependent average phonon number, where the time-dependence comes from the particular realization of the noise  $\xi_c(t)$ . Clearly, for times when  $|\xi_c(t)|$  is small, this becomes large, and vice versa.

If we now ensemble average  $\langle b^\dagger(t)b(t) \rangle_{r(t)}$  over the noise  $\xi_c(t)$ , the realizations where  $r(t)$  is small will contribute the most, such that the full ensemble average (or long time average) should become larger than the result  $n_m^{(\text{QNA})}$  from the quantum noise approach, since  $\langle 1/(c + dr^2) \rangle > 1/(c + d\langle r^2 \rangle)$ , but still smaller than  $n_m^T$ .

### a. Amplitude distribution function

We assume that the classical and complex  $\xi_c(t)$  is drawn from a Gaussian probability distribution with zero mean, i.e., it is distributed according to

$$\tilde{P}(\xi_c) = \frac{1}{\mathcal{N}} e^{-k|\xi_c|^2}, \quad (\text{S60})$$

where  $k$  is a constant to be determined and  $\mathcal{N}$  is a normalization constant. Transforming to polar coordinates and integrating over the polar angle gives the probability distribution over amplitudes  $r = |\xi_c|$ :

$$P(r) = r \int_0^{2\pi} d\varphi \tilde{P}(re^{i\varphi}) = \frac{2\pi}{\mathcal{N}} r e^{-kr^2}, \quad (\text{S61})$$

where the additional factor of  $r$  comes from the Jacobian determinant. We note that, even though  $\xi_c$  has zero mean, i.e., there is no phase coherence of the incoming noise, the amplitude  $r > 0$  does not have zero mean and does not obey Gaussian statistics.

Let us first determine the normalization constant  $\mathcal{N}$  by requiring

$$\int_0^\infty dr P(r) = 1, \quad (\text{S62})$$

giving

$$\mathcal{N} = \frac{\pi}{k} \quad (\text{S63})$$

such that

$$P(r) = 2kre^{-kr^2}. \quad (\text{S64})$$

We can now determine the constant  $k$  from Equation (S43), i.e., by requiring that

$$\langle r^2 \rangle = \int_0^\infty dr r^2 P(r) = F_0. \quad (\text{S65})$$

This gives

$$k = \frac{1}{F_0}, \quad (\text{S66})$$

i.e., the width of the Gaussian (S60) is given by the incoming flux  $F_0$ .

### b. Average phonon number

Let us now calculate the phonon number  $n_m$  averaged over different realizations of the incoming noise, i.e., the average of Equation (S59). We can then express the phonon number as

$$n_m = n_m^T \tilde{I}(k, q), \quad (\text{S67})$$

where we have defined the integral

$$\tilde{I}(k, q) = \int_0^\infty dr \frac{1}{1 + qr^2} P(r) = 2k \int_0^\infty dr \frac{re^{-kr^2}}{1 + qr^2} \quad (\text{S68})$$

and the constant

$$q = \frac{4g_0^2}{\gamma\omega_m^2}. \quad (\text{S69})$$

By a change of variables  $u = qr^2$ , we can transform the integral to

$$\tilde{I}(k, q) = \lambda \int_0^\infty du \frac{e^{-\lambda u}}{1+u} \equiv I(\lambda) \quad (\text{S70})$$

when defining

$$\lambda = \frac{k}{q} = \frac{\gamma}{\gamma_{\text{opt}}}, \quad (\text{S71})$$

where  $\gamma_{\text{opt}}$ , defined as in Equation (S44), is the optomechanical damping one would have with coherent driving with flux  $F_0$ , as before.

To our knowledge, it is not possible to find an analytical expression for the integral  $I(\lambda)$  in (S70), although it is possible to express it as

$$I(\lambda) = \lambda e^\lambda \Gamma(0, \lambda), \quad (\text{S72})$$

where

$$\Gamma(s, x) = \int_x^\infty t^{s-1} e^{-t} \quad (\text{S73})$$

is the *upper incomplete gamma function*. However, we may proceed by considering the (most interesting) regime

$$\lambda \ll 1, \quad (\text{S74})$$

i.e., what would correspond to the damping being dominated by the optomechanical interaction in the case of coherent driving. We start by rewriting the integral as

$$I(\lambda) = \lambda^2 \int_0^\infty du \ln(1+u) e^{-\lambda u} \quad (\text{S75})$$

which follows from partial integration. We now assume that the integral is dominated by large values  $u \gg 1$  for  $\lambda \ll 1$ . We may then approximate the integrand such that

$$\begin{aligned} I(\lambda) &\approx \lambda^2 \int_0^\infty du \ln u e^{-\lambda u} \\ &= \lambda \int_0^\infty dx (\ln x - \ln \lambda) e^{-x}. \end{aligned} \quad (\text{S76})$$

By introducing *Euler's constant*

$$C = - \int_0^\infty dx \ln x e^{-x} = 0.5775772156649..., \quad (\text{S77})$$

we now find

$$I(\lambda) \approx \lambda (\ln \lambda^{-1} - C). \quad (\text{S78})$$

By inserting (S78) into (S67), we then arrive at an analytical expression for the phonon number in the limit where the noise bandwidth is much smaller than the thermal equilibration rate:

$$n_m = \frac{\gamma n_m^T}{\gamma_{\text{opt}}} \left[ \ln \left( \frac{\gamma_{\text{opt}}}{\gamma} \right) - C \right]. \quad (\text{S79})$$

We observe that this satisfies

$$\frac{\gamma n_m^T}{\gamma_{\text{opt}}} < n_m < n_m^T, \quad (\text{S80})$$

i.e., its value lies between the wide bandwidth (or coherent driving) phonon number and the thermal bath occupation number, as expected.

### c. Average spectrum and effective mechanical linewidth

Let us now define the mechanical spectrum for a particular fixed value of the noise amplitude  $r$  as

$$\begin{aligned} S_r(\omega) &= \int_{-\infty}^\infty d\tau e^{i\omega\tau} \langle b^\dagger(t+\tau) b(t) \rangle_r \\ &= \frac{\gamma n_m^T}{[(\gamma + \gamma_{\text{opt}} r^2 / F_0) / 2]^2 + (\omega + \omega_m)^2} \end{aligned} \quad (\text{S81})$$

where we, as in the previous section, ignore the radiation pressure shot noise term for simplicity. For noise bandwidths smaller than the thermalization rate, the actual spectrum one would measure for sampling times much longer than the noise correlation time is

$$S(\omega) = \int_0^\infty dr S_r(\omega) P(r). \quad (\text{S82})$$

We first note that the area under the spectrum gives the average phonon number, since

$$\begin{aligned} \int_{-\infty}^\infty \frac{d\omega}{2\pi} S(\omega) &= \int_0^\infty dr P(r) \int_{-\infty}^\infty \frac{d\omega}{2\pi} S_r(\omega) \\ &= n_m^T I(\lambda) = n_m. \end{aligned} \quad (\text{S83})$$

Finding the explicit form of the average spectrum (S82) is not straightforward. However, let us attempt to *fit* it to a Lorentzian, i.e., let's write  $S(\omega) \approx L(\omega)$  with

$$L(\omega) = \frac{\gamma_{\text{eff}} n_m}{(\gamma_{\text{eff}}/2)^2 + (\omega + \omega_m)^2}. \quad (\text{S84})$$

It is straightforward to check that (S83) is satisfied in this approximation. We now fit the Lorentzian by *defining* the effective linewidth  $\gamma_{\text{eff}}$  such that the height of the Lorentzian matches the actual maximum of the spectrum, i.e., we demand

$$L(-\omega_m) = S(-\omega_m). \quad (\text{S85})$$

This means that

$$\begin{aligned} \frac{4n_m}{\gamma_{\text{eff}}} &= \int_0^\infty dr S_r(-\omega_m) P(r) \\ &= \frac{4n_m^T}{\gamma} \lambda \int_0^\infty du \frac{e^{-\lambda u}}{(1+u)^2} \end{aligned} \quad (\text{S86})$$

where  $\lambda$  is defined as before in (S71). Partial integration then gives

$$\begin{aligned} \frac{4n_m}{\gamma_{\text{eff}}} &= \frac{4n_m^T}{\gamma} \lambda \left[ 1 - \lambda \int_0^\infty du \frac{e^{-\lambda u}}{1+u} \right] \\ &= \frac{4(n_m^T - n_m)}{\gamma_{\text{opt}}}, \end{aligned} \quad (\text{S87})$$

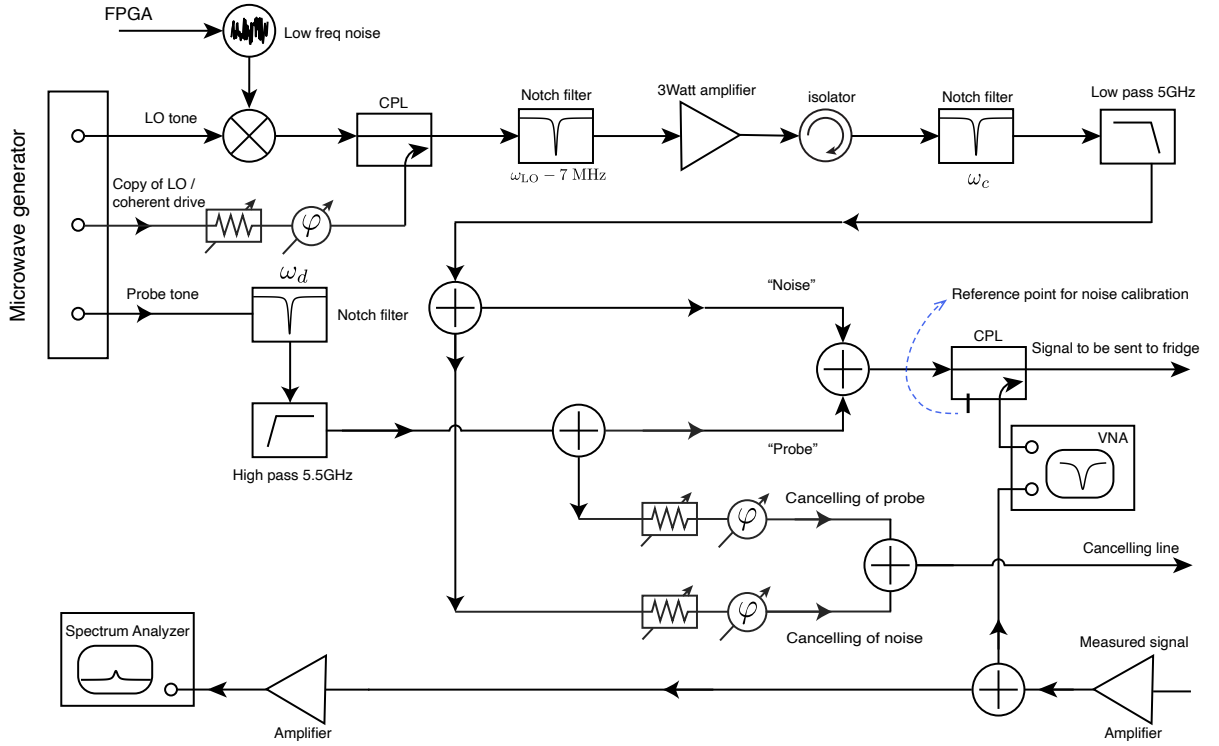

FIG. S2. Room temperature measurement setup. For discussion, see text.

such that

$$\gamma_{\text{eff}} = \gamma_{\text{opt}} \frac{n_m}{n_m^T - n_m}. \quad (\text{S88})$$

For  $n_m \ll n_m^T$ , this becomes

$$\gamma_{\text{eff}} = \gamma \ln \left( \frac{\gamma_{\text{opt}}}{\gamma} \right). \quad (\text{S89})$$

## II. EXPERIMENTAL SETTING

In this section, we discuss the experimental setup, mostly the room temperature setup that we use in the noise driving experiment, and detail the specific method of generating the band-limited noise centered at the red sideband of pump cavity mode.

### A. Noise generation

Here, we describe and justify the schematics drawn in Fig. S2. The low frequency noise is first created as a low-frequency (baseband) noise signal with a box function spectral profile. The simplest option would be to create low-pass filtered noise using a simple RF function generator, spanning from zero frequency up to some cut-off, and then up-convert it with the Local Oscillator (LO). However, this would result in two correlated images of the

baseband signal on either frequency side of the LO, possibly affecting the assumption of uncorrelated noise. For this reason, we decided to generate the baseband noise centered at a finite and relatively high frequency, here 7 MHz, with a sharp box-function spectral profile.

Standard function generators do not allow to generate such a specific spectrum. Furthermore, analog filtering of a low-pass filtered noise is not a suitable option, as standard analog filters do not provide steep enough roll-off. Therefore, we generate the noise signal using a sequence of  $30 \times 10^6$  Gaussian-distributed random values from a random number generator (Ziggurat method, provided by the GSL library for C++). We then perform digital filtering on these points to create a box-shaped spectrum centered at 7 MHz. After scaling and formatting operations, these points are loaded into the Dynamic Random Access Memory (DRAM) associated to a FPGA processor (Kintex-7 325T, in a NI FlexRIO PXIe-7972 module) to be played with a 16-bit resolution (over a range of  $\pm 2$  V) at a sampling frequency of 100 MHz, by the output channel of a transceiver associated to the FPGA card. The number of points used in this method of noise generation is limited by the size of the DRAM available on the FPGA module. The noise trace that is fed to the DRAM lasts 0.3 s, and it is repeated in a loop. This timescale is much longer than any other timescale of the sample. However, these constraints impose a lower bound on the bandwidth of noise that can be reliably generated in this manner, as the number of frequency points participating

in the bandwidth of noise becomes too low to establish a good statistics.

This noise is then mixed with the LO tone ( $\omega_{\text{LO}} = \omega_c - \omega_m - 7$  MHz) to place the upper sideband of the mixing at the red optomechanical sideband of the pump cavity. The mixer employed here is a single-sideband (SSB) mixer, which efficiently suppresses the generation of the lower sideband as long as it sits further away than 4 MHz from the LO frequency. In the experiment, the signal in upper and lower sidebands extends over bandwidths of up to 4 MHz: the center of the lower sideband should therefore sit at least 6 MHz away from the LO so as to use the attenuation provided by the SSB mixer to suppress the whole bandwidth of the lower sideband. We chose an even larger LO detuning from the optomechanical sideband, of 7 MHz, so as to allow for further filtering of the lower sideband using an analog notch filter without affecting the upper sideband. The single-sideband mixer then rejects the undesired image of the noise below the LO frequency by about 25 dB, and we further notch-filter the image, since otherwise possibly detrimental intermodulation products will appear.

In the mixing operation, the LO signal leaks through the mixer, which results in a coherent signal at  $\omega_{\text{LO}}$  also propagating towards the sample. The optomechanical contribution of this coherent signal is not too strong since it is substantially detuned from the sideband and partially filtered by the notch filter used to suppress the lower sideband of the noise. However, we eliminate further it to make sure that the cooling is due to the noise alone. Therefore, this tone is actively cancelled out by about 45 dB thanks to a destructive interference with a second tone of equal frequency generated by the same microwave generator (for phase stability), with an appropriate phase and amplitude. In all experiments, the power of the residual coherent tone is thus maintained at least 25 dB below the total integrated power of the noise.

The box-profiled microwave noise is then amplified by a 3 Watt power amplifier, and sent through a notch filter at the pump cavity frequency, and through a 5 GHz low pass filter. The role of the notch filter is to eliminate harmful noise at the cavity frequency that would pose strong limits on available cooling. The low pass filter serves to mitigate broadband noise from the power amplifier being injected to the probe cavity, which can introduce extra heating to the mechanics, or interference in the probing. The relatively weak coherent probe tone is also going through a notch filter and a high pass filter, for the same reasons as described immediately above.

Examples of the generated noise spectra are shown in Fig. S4 (a). We obtain sharp roll-off, about 9 dB per kHz even at the largest bandwidths.

The generated noise and coherent tone are combined with a power combiner and sent to the dilution refrigerator. Additionally, these two signals are split before the combiner to be sent through a separate line each containing a tunable amplitude attenuator and tunable phase shifter. As a result, the driving broadband noise and

probe tone can be cancelled inside the refrigerator after they are reflected from the sample before reaching the low temperature HEMT amplifier. Without such cancelling, we expect saturation of the HEMT or the last amplification stage at room temperature.

## B. Noise calibration

Throughout all experiments, to compare the optomechanical impacts of noise and of coherent signals, we ensured that the total integrated power of the noise is equivalent to the power of the coherent tones employed, and this whatever the bandwidth of the noise. In practice, we calibrate the ratio of noise power to a coherent tone power at given generator settings (see Section III A below). We realized calibration sweeps of the noise bandwidth and measured it after the whole signal conditioning chain as indicated by the calibration point marked in Fig. S2.

We found that the data stream from the FPGA already ensured that the power was constant within  $\pm 0.2$  dB at large bandwidths, but systematic variations up to 2.5 dB were seen at bandwidths  $< 500$  Hz, which can be attributed to the small available statistics on the distribution of the noise within this technique. This was taken into account in rescaling of the noise amplitude, allowing to maintain the final integrated power constant within  $\pm 0.5$  dB. This bandwidth-dependent rescaling does not patch the lack of statistics, but at least allows the noise with its imperfect statistics to be used for comparison to other driving situations.

Finally, noise power sweeps were also performed at fixed bandwidths to ensure that none of the elements of the microwave setup (mixers, amplifiers) are saturated by the range of powers used in the experiments.

## III. CALIBRATIONS AND DATA ANALYSIS

The sideband-cooling situation, where the pump is set at the frequency  $\omega_c - \omega_m$ , is the basis for most calibrations. Some forms of these measurements are carried out in both the pump and probe cavities. Below we will attempt to be clear which cavity is explicitly under consideration at a given point.

At this point that we are considering the emitted output field from the cavity, we have to split the cavity energy loss to the internal and external losses, which occur at the respective rates  $\kappa_i$  and  $\kappa_e$ , and sum up to  $\kappa = \kappa_i + \kappa_e$ . Similarly, it is necessary to take into account classical cavity noise in the probe cavity, described by the number of thermal photons  $n_c^T$ . The latter is due to technical heating by the microwaves applied to the sample.

In the good-cavity limit, and if the optical damping due to the coherent tone  $\Gamma_{\text{opt}} \ll \kappa$ , the output spectrum

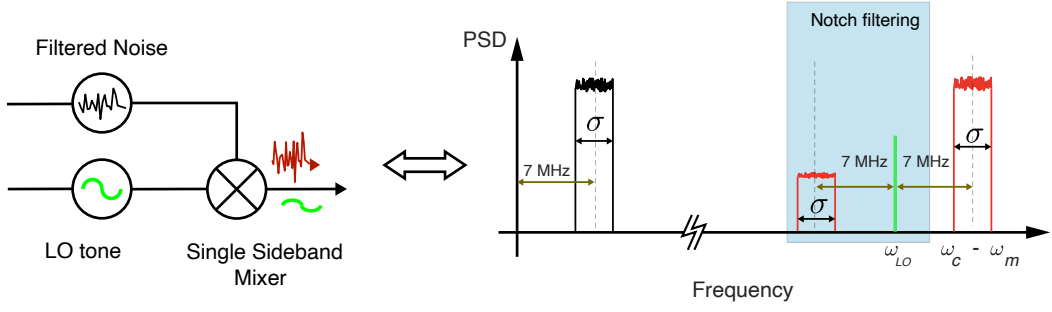

FIG. S3. *Noise generation.* For details, see text.

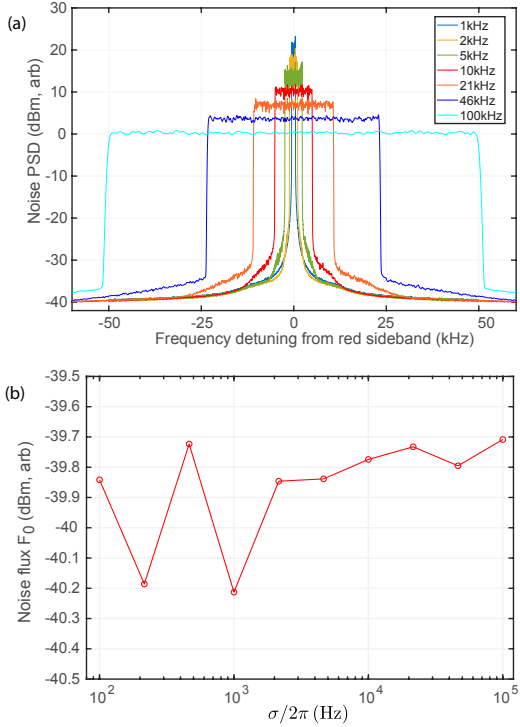

FIG. S4. *Noise calibrations.* (a) The spectral profiles of the noise sent to the sample is displayed at different bandwidths  $\sigma$  as indicated. (b) Integrated noise power as a function of bandwidth.

after amplification with gain  $\mathcal{G}$  satisfies

$$\frac{S_{\text{out}}[\omega]}{\mathcal{G}} = \frac{4\kappa_e}{\kappa} n_c^T + \frac{\kappa_e}{\kappa} \frac{\Gamma_{\text{opt}} \gamma_{\text{eff}}}{\omega^2 + \gamma_{\text{eff}}^2/4} (n_m - 2n_c^T) + n_{\text{add}}. \quad (\text{S90})$$

This includes a background level due to amplifier added noise  $n_{\text{add}}$ . The Lorentzian contains destructive interference between the classical cavity noise, and transduced mechanical motion. The interference leads to "noise squashing", and the peak in the output spectrum under nonzero cavity noise is not any more fully faithful reconstruction of the state of the mechanics. As we discuss below, the cavity noise has a minor but non-

negligible contribution in the thermometry.

### A. Noise flux calibration

As discussed in the main text, the noise-induced average photon number  $\bar{n}_0$  in the pump cavity is determined using a coherent tone applied in the pump cavity. This is the regular sideband cooling experiment, which is presented in Fig. S5.

The cavity photon number  $n_0$  under a coherent tone is proportional to generator power  $P$  with the proportionality constant  $\mathcal{K}$ :

$$n_0 = \mathcal{K}P. \quad (\text{S91})$$

The optical damping is then written as

$$\Gamma_{\text{opt}} = \frac{4g_0^2 n_0}{\kappa} = \frac{4g_0^2}{\kappa} \mathcal{K}P. \quad (\text{S92})$$

We perform a linear fit to the experimentally determined  $\Gamma_{\text{opt}}$  as a function of the generator power, obtaining the calibration constant  $\mathcal{L}$ ,

$$\Gamma_{\text{opt}} = \mathcal{L}P, \quad (\text{S93})$$

and comparison with Eq. (S92) yields the important calibration coefficient:

$$\mathcal{K} = \mathcal{L} \frac{\kappa}{4g_0^2}. \quad (\text{S94})$$

We now use this calibration for noise driving. Cavity noise photon number is proportional to the noise generator power, but with a different proportionality constant  $\mathcal{K}_n = \beta\mathcal{K}$ , which we wrote in terms of  $\beta$  which is the correction factor coming from differences in synthesis, e.g.,  $\beta < 1$  means that noise power is smaller than coherent power at given generator setting. The noisy photon number becomes

$$\bar{n}_0 = \mathcal{K}_n P_n = \beta \mathcal{K} P. \quad (\text{S95})$$

The value of  $\beta$  is determined by measuring the ratio of coherent power and noise power going into the refrigerator:

$$\beta = \frac{\mathcal{K}_n}{\mathcal{K}} = \frac{\bar{n}_0}{n_0}, \quad (\text{S96})$$

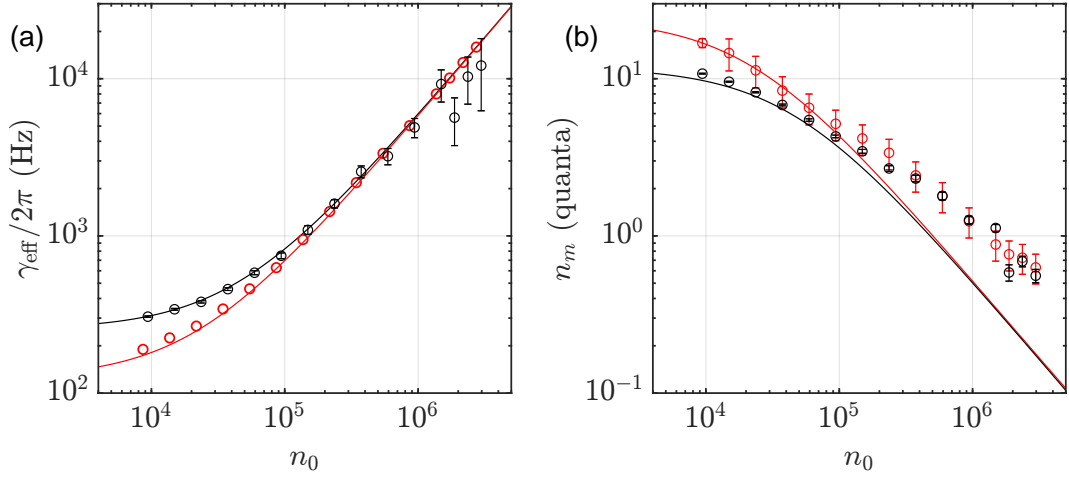

FIG. S5. *Sideband cooling calibration with a coherent tone.* The graphs are analogous to those in Fig. 2 in the main text. The color coding corresponds to inference from output spectrum from the pump cavity with the probe-cavity tone off (red), and detection from the probe cavity (black). The solid lines are the corresponding theoretical predictions. (a) Effective damping. The value from the pump cavity data (red) is smaller than the probe value (black) at small power because of the lack of the residual cooling by the probe tone. (b) Mechanical occupation. The theoretical graphs do not include any technical heating.

and the noise power calibrated with coherent tone is

$$\bar{n}_0 = \beta \mathcal{K} P = \beta \mathcal{L} \frac{\kappa}{4g_0^2} P_n \quad (\text{S97})$$

### B. Thermometry calibration

The thermometry calibration involves several steps which are discussed below. In this section, we exclusively treat the probe cavity, which is used for the thermometry. The optical damping  $\Gamma_{\text{opt}}$  below is thus that due to effective coupling  $G_d$ .

With the thermometry, we primarily work with the corresponding integrated peak area on top of the background level set by amplifier noise and possible cavity noise. For simplicity, we also include the transduction factor  $\frac{\kappa_e}{\kappa}$  into the definition of the system gain  $\mathcal{G}$ . We obtain from Eq. (S90)

$$A_{\text{out}} = \int S_{\text{out}}[\omega] d\omega = 2\pi \mathcal{G} \Gamma_{\text{opt}} (n_m - 2n_c^T). \quad (\text{S98})$$

The peak area thus acts as a thermometer, containing the occupation number  $n_m$ , transduced at the efficiency given by the probe power contained in  $\Gamma_{\text{opt}}$ . Notice that in this measurement, the mode occupation  $n_m$  depends on the probe power, which needs to be carefully addressed at the calibration stage.

From Eq. (S98) we see that due to the noise squashing, the peak area can be eaten away by the cavity noise, and can even turn negative. To include this effect in the calibration, we separately measure  $n_c^T$  by recording the background noise level (see Eq. (S90)) with all or some of the microwaves switched off, and study the background level raise during the actual operations.

In the thermal calibration, the refrigerator temperature is stepped over a large range. In this measurement, we find that  $n_c^T$  is negligible since a very small microwave power was used. The peak area is then written as

$$A_{\text{out}} = \frac{2\pi \mathcal{G} \gamma \Gamma_{\text{opt}}}{\gamma_{\text{eff}}} n_m^T = \underbrace{\frac{2\pi \mathcal{G} \gamma \Gamma_{\text{opt}} k_B}{\gamma_{\text{eff}} \hbar \omega_m}}_{\equiv \mathcal{T}} T = \mathcal{T} \frac{\hbar \omega_m}{k_B} n_m^T. \quad (\text{S99})$$

A linear temperature dependence is fitted to the measured peak area to recover the calibration coefficient  $\mathcal{T}$ . The mechanical bath occupation (different from mode temperature  $n_m$ ) is then established as

$$n_m^T(T) = \frac{k_B}{\mathcal{T} \hbar \omega_m} A_{\text{out}}(T). \quad (\text{S100})$$

An important calibration figure, the equilibrium thermal occupation  $n_{m,0}^T$  under the operation temperature  $T_0$ , is  $n_{m,0}^T = n_m^T(T_0)$ . In the experiment, we operate near the base temperature of the refrigerator, with  $T_0 \simeq 10$  mK. The temperature sweep is shown in Fig. S6 (a), where we find  $n_{m,0}^T = 24.2 \pm 1.2$ .

Next, we carry out a standard sideband cooling measurement via the probe cavity, by stepping the probe power over a large range. Equation (S90) is collectively fitted to the spectral profiles, by using the gain as a collective adjustable parameter, and  $n_m^T$  as an adjustable parameter for each trace individually. Here, we implement the obtained value of equilibrium thermal occupation  $n_{m,0}^T$  as fixing  $n_m^T$  values for low-power traces, where possible technical heating is negligible, instead of relaxing it as a fitting parameter as is done for the remaining traces. The obtained results for the occupation  $n_m$  and peak area are shown in Fig. S6 (b).

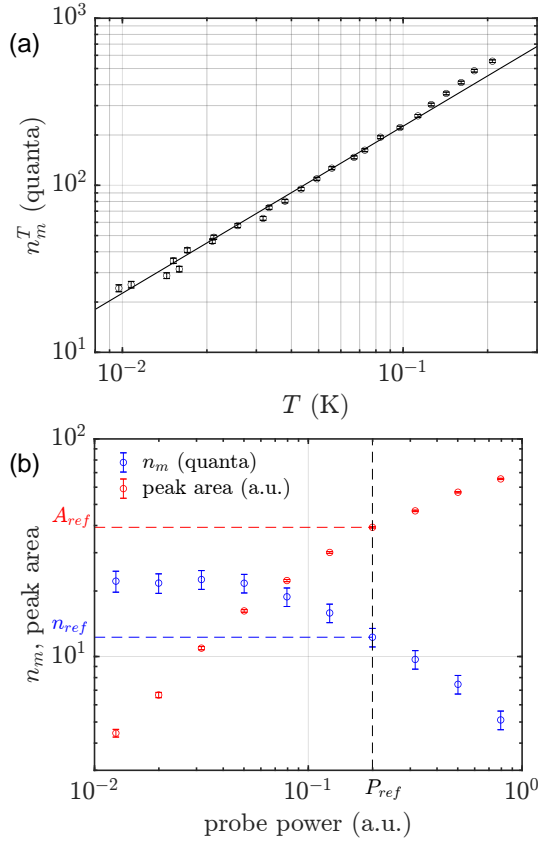

FIG. S6. *Thermometry calibration.* (a) hermal sweep at a small cooperativity, together with a linear fit according to Eq. (S99). (b) Sideband cooling calibration via the probe cavity. The relations of the calibration values for mechanical occupation and peak area are indicated by the dashed lines.

We then select a suitable probe power  $P_{\text{ref}}$ , which we use in all subsequent thermometry. The power value is selected high enough such that sufficient signal is obtained, but small enough such that the probe itself does not induce excessive sideband cooling. We again find that the cavity noise  $n_c^T$  is negligible. The relation between thus obtained reference values for the peak area  $A_{\text{ref}}$  and occupation  $n_{\text{ref}}$  at a given power is from Eq. (S98)

$$A_{\text{ref}} = 2\pi\mathcal{G}n_{\text{ref}}\gamma_{\text{ref}}. \quad (\text{S101})$$

This process is described in Fig. S6 (b).

The thermometry reading, when the same probe power is used as in Eq. (S101) is then obtained by dividing Eq. (S98) by Eq. (S101):

$$n_m = n_{\text{ref}} \frac{A_{\text{out}}}{A_{\text{ref}}} + 2n_c^T. \quad (\text{S102})$$

In the cooling experiments, where high powers are applied to the pump cavity, we find that the probe cavity exhibits non-negligible noise raise up to  $n_c^T \simeq 0.06$ , see Fig. S7.

### C. Error estimation

The uncertainty of the thermometry, Eq. (S102), is due to uncertainties in the included variables  $n_{\text{ref}}$ ,  $A_{\text{out}}$ , and

$A_{\text{ref}}$ . That of  $n_c^T$ , whose value has only a small influence on the occupation, becomes negligible.

Those of the measured peak areas,  $A_{\text{out}}$  and  $A_{\text{ref}}$ , are the statistical errors of determination of the peak area from the spectra. These are obtained via the standard error of the weighted residual

$$\sigma_r = \sqrt{\frac{\sum_{n=0}^N [S(\omega_n) - S^{th}(\omega_n)]^2}{N} H(\omega_n)} \quad (\text{S103})$$

Here,  $N$  is the number of data points in a given trace,  $\omega_n$  are the frequency values,  $S(\omega_n)$  are the measured data points, and  $S^{th}$  is a Lorentzian least-square fit function. The weighting  $H = \frac{S^{th}(\omega_n)}{\max(S^{th})}$  in Eq. (S103) implies that the focus is in the peak region, while long tails of the Lorentzian give no weight to the numerical integration.

The uncertainty of the peak area, in other words, of the sum  $\sum_{n=0}^N S(\omega_n)$ , is obtained as  $\sqrt{N}\sigma_r$ , which corresponds to  $\sigma$  error bars.  $2\sigma$  error bars, which we use, are then

$$dA_{\text{out}/\text{ref}} = 2\sqrt{N}\sigma_r \quad (\text{S104})$$

The uncertainty of the reference occupation  $n_{\text{ref}}$  involves two significant contributions. One is the statistical error in the described sideband cooling fitting, and the other is the error in determining  $n_m^0$ .

All error contributions are propagated quadratically to yield the final uncertainty estimates. The clearly dominant error source in thermometry is the statistical error of determining the area of the very small peak.

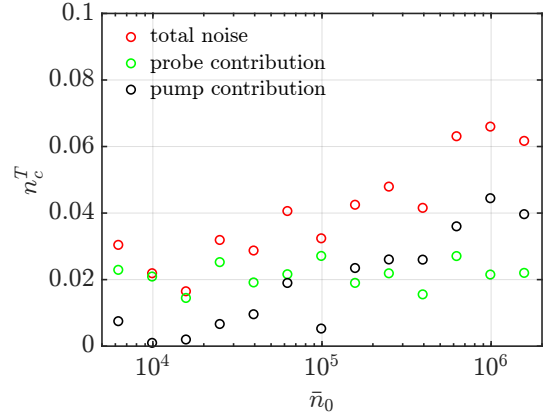

FIG. S7. *Heating in the probe cavity.* Noise flux inducing the given photon number  $\bar{n}_0$  is applied to the pump cavity. The total probe cavity noise (red) can be divided into contributions due to the probe tone (green), and to the pump tone (black), by keeping on only one tone, both tones, or neither. This is the same dataset shown in Fig. 2 in the main text.

- 
- [1] A. A. Clerk, M. H. Devoret, S. M. Girvin, F. Marquardt, and R. J. Schoelkopf, Introduction to quantum noise, measurement, and amplification, *Rev. Mod. Phys.* **82**, 1155 (2010).
  - [2] F. Marquardt, J. P. Chen, A. A. Clerk, and S. M. Girvin, Quantum theory of cavity-assisted sideband cooling of mechanical motion, *Phys. Rev. Lett.* **99**, 093902 (2007).
  - [3] I. Wilson-Rae, N. Nooshi, W. Zwerger, and T. J. Kippenberg, Theory of ground state cooling of a mechanical oscillator using dynamical backaction, *Phys. Rev. Lett.* **99**, 093901 (2007).
